# Supplementary material for: DoGR: Disaggregated Gaussian Regression for Reproducible Analysis of Heterogeneous Data
Source: arXiv:2108.13581 source file (2021-08-31)
Supplement: Supplementary file 1 [file appendix.tex]

\appendix
\section{Connection to joint distribution\label{apndx:connection}}
Here we show that multiplication of $f_{Y | X}(y|x) f_{X}(x)$ could be converted to a normal distribution. 
$$f^{(k)}_{X, Y}(x, y) = f_{Y | X}(y|x) f_{X}(x) = \varphi(y; \beta_k X, \sigma_k) \varphi(x; \mu_k, \Sigma_k)$$
\begin{flushleft}
$f^{(k)}_{X, Y}(x, y) =$\\
\end{flushleft}
%\begin{flushright}
$$\frac{\text{exp}\{ \frac{-1}{2} (x - \mu_k)^T \Sigma_k^{-1} (x - \mu_k)\}}{\sqrt{(2\pi)^D |\Sigma_k|}}  \times \frac{\text{exp}\{\frac{-(y - \beta_k x)^2}{2 \sigma_k^2}\}}{\sqrt{2\pi \sigma_k^2}}$$
%\end{flushright}
\begin{flushleft}
$f^{(k)}_{X, Y}(x, y) = $
\end{flushleft}
$$\frac{\text{exp}\{ \frac{-1}{2} [(x - \mu_k)^T \Sigma_k^{-1} (x - \mu_k) + (y - \beta_k x) \sigma_k^{-2} (y - \beta_k x)] \}}{\sqrt{(2\pi)^{D+1} |\Sigma_k| \sigma_k^2}}$$

So finally, 

$$f^{(k)}_{X, Y} \sim \mathcal{N}(\mu'_k, \Sigma'_k)$$

Where $\mu'_k = [\mu_k^{(1)}, \mu_k^{(2)}, ..., \mu_k^{(d)}, \beta_k X]$ and $\Sigma'_k = \left[{\begin{array}{cc} \Sigma_k & 0 \\ 0 & \sigma_k \\ \end{array} } \right]$ is a block matrix.
